# Supplementary material for: Direct observation of homogeneous cavitation in nanopores
Source: arXiv:2007.03521 source file (2020-12-14)
Supplement: Supplementary file 1 [file Doebele_HomogeneousCavitationMembranes_SM.pdf]

# Supplemental Material for
# Direct observation of homogeneous cavitation in nanopores

V. Doebele,[1] A. Benoit-Gonin,[1] F. Souris,[1] L. Cagnon,[1] P. Spathis,[1] P.E. Wolf,[1,*]
A. Grosman,[2,†] M. Bossert,[2] I. Trimaille,[2] C. Noûs,[3] and E. Rolley[4,‡]

[1]*Université Grenoble Alpes, CNRS, Institut Néel, F-38042 Grenoble, France*

[2]*Sorbonne Université, CNRS, Institut des NanoSciences de Paris, INSP, F-75005 Paris, France*

[3]*Laboratoire Cogitamus 1 3/4 rue Descartes, 75005 Paris*

[4]*Laboratoire de Physique de l'Ecole Normale Supérieure, ENS, Université PSL, CNRS, Sorbonne Université, Université de Paris, F-75005 Paris, France*

(Dated: October 16, 2020)

## CONTENTS

Overview 2

Sample preparation 3

Porous alumina membranes 3

Porous silicon membranes 4

Alumina deposition 5

Upper bound for the diameter of constrictions 7

Membranes deformation 7

Experimental set-up 8

Measuring the liquid fraction 8

Dependence of the evaporation pressure in porous silicon on the cavity geometry 11

Detection of cavitation in alumina membranes by optical transmission measurements 12

Comparison to bulk CNT for porous alumina and discussion of experimental errors 16

References 18

## OVERVIEW

This Supplemental Material provides details on the experimental methods used in our paper, and on the analysis of the results. We first describe the fabrication of our ink-bottle pores, and estimate an upper bound for the obtained constriction diameters. We also discuss the possible effect of the membrane deformation on our results. We then detail our experimental set-ups, and show that the liquid fraction obtained from White Light Interferometry coincides with the result of conventional volumetric measurements. In the following section, we detail the effect of the cavity size on the evaporation pressure in porous silica membranes. The next section supports Fig.4 of the paper by describing how measurements of the poAl membranes optical transmission allow to track condensation and evaporation. Figure 8 presents the analog of the inset of Fig.4 of the paper for the 25 nm membrane.

Finally, we justify why cavitation in alumina membranes can be compared to bulk CNT, and discuss the influence of the various experimental errors.

## SAMPLE PREPARATION

### Porous alumina membranes

The nanoporous alumina membranes have been fabricated using the two-step anodizing procedure in mild conditions introduced by Masuda et al[1]. The starting material consists of high purity 2 inch diameter aluminum disks (99.999%, Goodfellow) that were first, mechanically polished to mirror-like aspect, and second, electropolished in an ethanol:perchloric acid mixture (4:1 in volume) at 0°C and 30 V for 2 minutes, leading to bright and shiny surfaces.

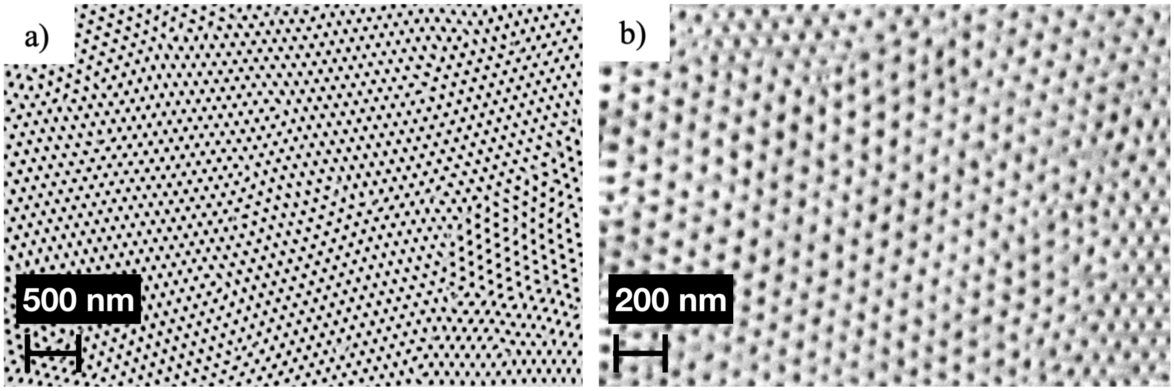


FIG. 1. SEM top views of alumina membranes anodized in (**a**) 0.5 M oxalic acid at 40 V , and (**b**) 0.3 M sulfuric acid at 25 V.

PoAl membranes with wide and narrow pores were respectively obtained by anodization in 0.5 M oxalic or 0.3 M sulfuric acid solutions [2, 3]. A platinum plate acts as a cathode and the bath temperature is regulated with a chiller. For oxalic acid electrolyte, the anodizing is done at a voltage of 40 V and a temperature 15°C. The first and second anodizing step durations are 17 h and 7 h respectively. For sulfuric acid electrolyte, the voltage and temperature were 25 V and 0°C. First and second step durations were 24 h and 20 h respectively. The alumina layer obtained after the first anodizing step is chemically etched in 0.2M $CrO_3$ + 0.4M

$H_3PO_4$ solution at 50°C prior to the second anodization. Finally, the underlying aluminum substrate is removed in $CuCl_2$ + HCl solution, leaving the alumina barrier layer intact, *i.e.* yielding a membrane with pores closed on one side and with a typical thickness of 60 to 100 microns. One centimeter side square samples were cut from these membranes and used for experiments or characterization. The pore diameter distribution on the open side of the membranes was determined by analyzing SEM images of samples after evaporating a 2 nm thick layer of gold [4]. After due correction for the gold thickness, the corresponding average pore diameters for different samples lie between 50 and 55 nm for membranes produced in oxalic acid, and 25 to 30 nm for those produced in sulfuric acid. The typical distribution width over the field of view of the SEM images is about 2 nm (Figure 1). Analyses of hexane sorption isotherms measured on such native membranes reveal that the pores are both conical in shape, wider at their open end than at their closed end, and corrugated [4]. As a result, the average pore volume, an important parameter in view of the comparison to the CNT, cannot be obtained from the knowledge of the membrane thickness and the average diameter at the pore open end only. Instead, we measure this volume by dividing the volume of liquid hexane which can be condensed into the native membranes (see below) by the total number of pores, estimated from the membrane's area and the interpore distance, precisely measured on SEM images (see table I). Dividing this volume by the pore length (equal to the membrane thickness, the alumina layer barrier thickness being less than 100 nm) determined by SEM gives the average pore area, from which we deduce an average diameter. For the two membranes of Fig. 4 of the paper, these diameters are respectively 60 and 25 nm, with a total estimated error around 15%.

**Porous silicon membranes**

Porous silicon membranes were synthesized by electro-etching p+-doped Si wafers in HF-ethanol solutions. We have used exactly the same doping and etching conditions as in Ref. 5, so the pores diameters and lengths are taken from previous measurements. Most samples used in the experiments have a porosity of 70% ($d$ in the range 12-40 nm, $\langle d \rangle = 25$ nm). In some cases, we used a sample of 85% porosity ($d$ in the range 23-80 nm, $\langle d \rangle = 50$ nm).

Duplex poSi samples were synthesized by etching in a Si wafer, first a 20 $\mu$m thick layer with small pores which act as constrictions ($\langle d \rangle \simeq 12$ nm), then a second layer of larger

| Figures | Thickness ($\mu$m) | Interpore spacing (nm) | Volume ($mm^3$) | Area ($cm^2$) | Porosity | Pore volume ($m^3$) | Diameter (nm) |
|---|---|---|---|---|---|---|---|
| 2,4, SI4 | 57 | 103 | 1.8 | 1 | 0.32 | 1.7e-19 | 61 |
| SI4 | 90 | 67 | 2.6 | 2.25 | 0.13 | 4.5e-20 | 25 |
| 4,SI8 | 75 | 67 | - | 1 | - | 3.7e-20 | (25) |

TABLE I. Geometrical characteristics of the alumina membranes used in the different figures of the paper. The thickness is measured from side view SEM images, the average interpore distance from top view SEM images. The total porous volume is measured by continuous volumetry as described in the text for the two first membranes (Fig. 4). The porosity, pore volume, and average diameter are computed from the previous values. For the third membrane, the total pore volume has not been measured, and the average diameter is taken equal to that of the second membrane, consistent with SEM pictures.

pores where cavitation-like evaporation occurs ($\langle d \rangle \simeq 26$ or 50 nm, $l = 4$ to 60 $\mu$m).

### Alumina deposition

Starting from the native membranes above, two different techniques were used to reduce the pore aperture. In the first one, used for the 60 nm poAl and the poSi membranes, we evaporate a 2 nm Al layer on the porous sample under 45° incidence angle, then oxidize this layer by exposing it to air at atmospheric pressure during 15 minutes. This step is repeated up to 12 times for the 60 nm poAl. Between each step, the sample is rotated by 90° around the pore axis, so that the deposition at the pore aperture is roughly isotropic. The vacuum chamber being pumped at each step, this procedure is quite time consuming.

A faster alternative technique, used for the 25 nm poAl membrane, relies on atomic layer deposition (ALD). The ALD reactor (Cambridge Nanotech Savannah S100) was kept at 250°C with a base pressure less than 1 Torr and nitrogen was used as a carrier gas with a flow rate of 5 standard $cm^3$ per minute. Alumina was deposited using trimethylaluminum (TMA) and water. In order to avoid extended diffusion of the precursors inside the nanopores, the reactor was operated in continuous mode, *i.e.* with the reactor chamber under continuous pumping. The precursors pulse duration was 15 ms with a purging time of 5 s in between

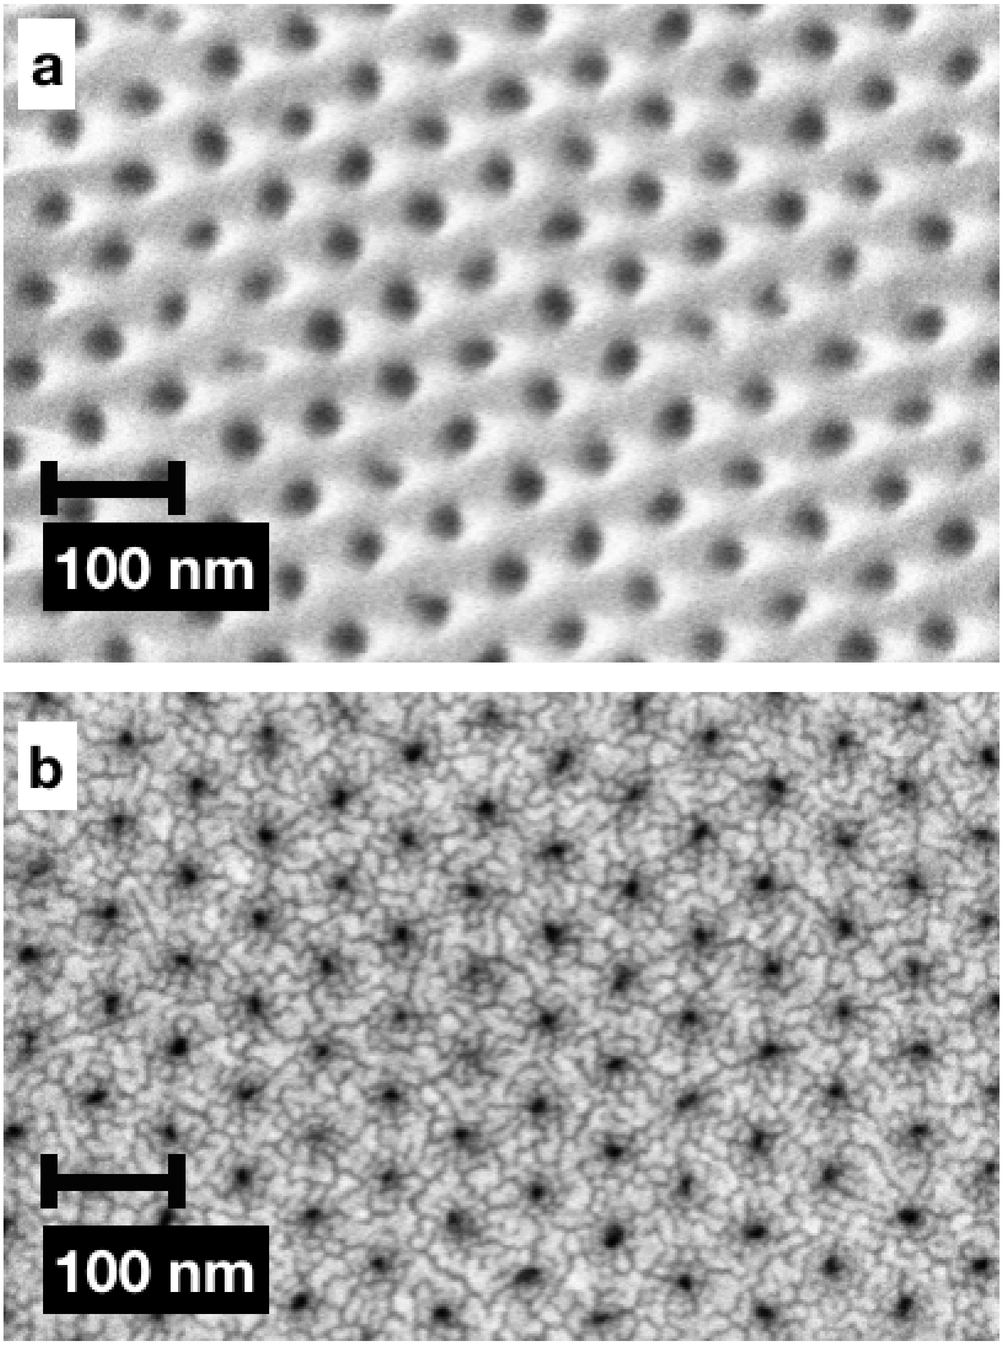


FIG. 2. SEM images of the top surface of alumina membranes (**a**) in the native state, average pore aperture around 30 nm (**b**) after 100 cycles of alumina deposition using Atomic Layer Deposition.

TMA and water pulses. In these conditions, the growth rate per cycle is 0.1 nm, which reduces the pore diameter by twice this quantity. Alumina is then only deposited at the pore aperture, resulting in the formation of the desired constriction. Figure 2 shows SEM images for poAl membranes with an average aperture of 30 nm, in the native state and

after 100 ALD cycles. The expected reduced aperture is around 8 nm, slightly less than the upper bound of 10 nm estimated from SEM. For the 25 nm diameter poAl pores, we had to deposit around 120 layers (nominal diameter reduction of 24 nm) to observe cavitation for half of the pores (the other being totally blocked). The corresponding pores aperture, expected to be of order of 5 nm at most, could be hardly distinguished on the SEM images (data not shown).

### Upper bound for the diameter of constrictions

The observation of cavitation in alumina implies that the evaporation pressure inside the constrictions is smaller than $P_{\mathrm{V}} \approx 0.33 P_{\mathrm{sat}}$. In order to convert the latter value to a maximal diameter for the constrictions, we use the Saam and Cole model [11] which assumes a van der Waals interaction between hexane and alumina. Estimating the alumina-hexane Hamaker constant $H$ as the geometric mean [12] of the hexane-hexane [13] and alumina-alumina [12] Hamaker constants, we find $H \approx 4.10^{-20}$J, corresponding to a van der Waals interaction strength of the order of 6.4 $10^4$ K.Å$^3$. Using this number, we find a maximal constriction diameter of 6 nm, consistent with the upper bounds deduced from SEM images.

### Membranes deformation

Along an isotherm, the porous stucture is submitted to capillary stresses of the order of 10 MPa. Such stresses can deform the porous material and affect the cavitation process. We have characterized the deformation in detail for porous silicon [6–8]. For the 70% porosity poSi samples mainly used in the present work, the deformation is of the order of $10^{-3}$. For the alumina membranes, the porosity is notably smaller than for poSi (table I) , and the elastic moduli of bulk alumina are larger than those of bulk silicon, so that the deformation of porous alumina membranes is expected to be below $10^{-3}$.

Such a small deformation could have an impact on the cavitation threshold if the pores were closed, as is the case in the experiments by Zheng et al. [9] and Azouzi et al. [10]. In this type of experiment, cavitation is obtained by decreasing the temperature of a closed inclusion so that the cavitation threshold can be strongly affected by a deformation of the matrix. In contrast, the pores in our system are open: the liquid inside is in equilibrium

with the vapor and the chemical potential is fixed. The pore volume of the pores then plays a role only through the number of nucleation sites, which enters only through a logarithmic factor in the cavitation pressure: the deformation can thus be safely neglected.

## EXPERIMENTAL SET-UP

The different curves of the paper have been obtained using two different set-ups, one at LPENS, and the other at Institut Néel. In both set-ups, condensation and evaporation are controlled in a similar way, depicted in Fig. 3.

The sample is enclosed in an optical cell with one or two windows. It is connected by one capillary line to a pressure gauge and can be filled or emptied through a second line. The latter is connected through a precision microvalve (Pfeiffer EVR116) to a pressure reservoir, consisting in a tank of liquid hexane immersed in a temperature-controlled bath. The cell temperature is regulated 2 °C below the room temperature to about 1 mK. For condensation, the bath temperature is set between the cell temperature and the ambient temperature to avoid condensation of liquid in the capillary lines. For poAl, depending on the pore diameter, the condensation pressure inside the membrane is typically 20-30 mbar below the tank saturation pressure. Evaporation is obtained by connecting the microvalve to a pump instead of the tank. Figures 4(a) and b show time traces of pressure in the cell as it is alternatively connected to the tank or to the pump, both for a native membrane and a membrane after deposition. Condensation or evaporation in the membrane are evidenced through a flattening of the time dependence of pressure. In order to avoid transient effects, we set the microvalve in such a way that the duration of the quasi-plateau is of order several hours, corresponding to a flow rate of order 0.2 STP $cm^3/h$ or less, for both condensation and evaporation. Note that such small flowrates cannot be precisely obtained and measured by commercial regulated flowmeters.

## MEASURING THE LIQUID FRACTION

The membrane liquid contents was measured as a function of pressure using two different methods. The first one, used at LPENS for both poAl and poSi, is reflection White Light Interferometry (WLI) [17, 18], which provides an instantaneous measurement of the mem-

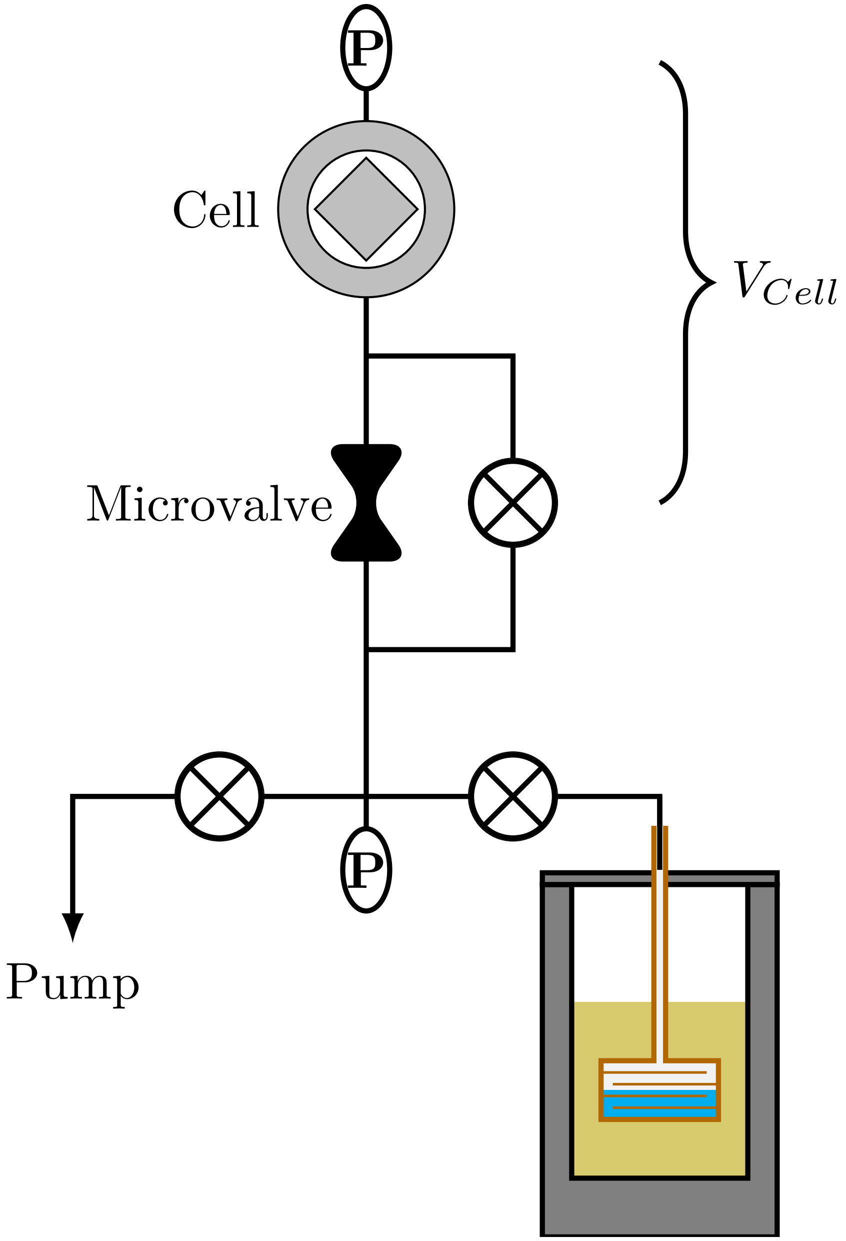


FIG. 3. Set-up used to control the condensation and evaporation of hexane.

brane average refractive index on a local scale ($\simeq$ 10 mm$^2$ area). Assuming this index to be a volume-weighted average of the bulk material (1.766 for alumina) and hexane (1.376) indexes, the change in the refractive index can be converted to the amount of condensed liquid. The result is quite close to that obtained using the more exact Bruggeman's approximation. For example, referring to Fig.2 of the paper, the total change of 0.12 corresponds to a porosity of 31%. The 0.01 value found just below the sharp condensation corresponds to a relative film fraction of ≈10%, the remaining 90% condensing over a narrow pressure

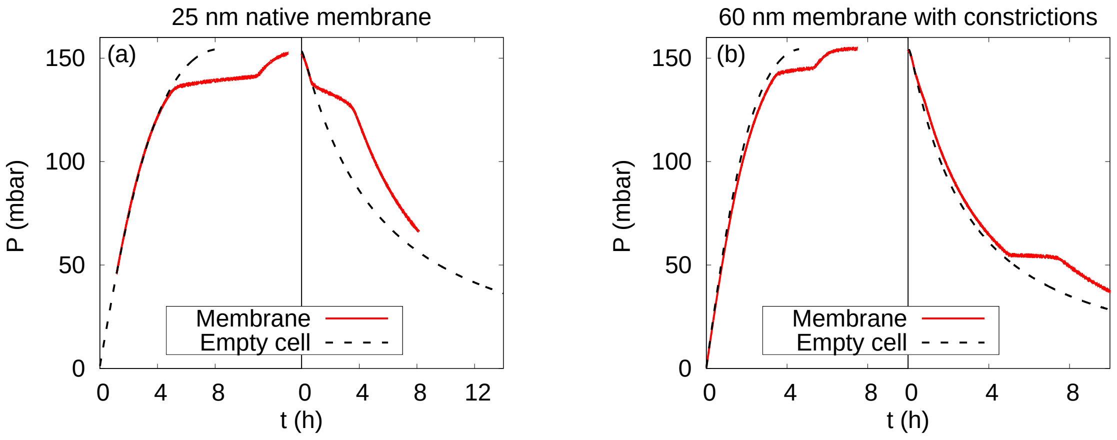


FIG. 4. Time dependence of the cell pressure during condensation and evaporation, for (**a**) a native 25 nm poAl membrane, and (**b**) the 60 nm poAl membrane of Figs. 2 and 4 of the paper. In both cases, the cell temperature is 19°C, corresponding to the same bulk saturation pressure $\simeq$ 155 mb. For condensation, the reservoir pressure is 170 mbar. Dashed lines correspond to the behavior measured without any membrane (a scaling factor on time has been applied to compensate for a different opening of the microvalve between the experiments with and without the membranes). As expected, the membrane with 25 nm pores condenses at a lower pressure than the membrane with 60 nm diameter pores. For the native membrane, evaporation takes place at a lower pressure than condensation. This hysteresis is interpreted as a signature of pore roughness [4, 14–16]. The longer duration of the condensation plateau compared to that of the evaporation plateau reflects a smaller flowrate (due to the smaller difference of pressures across the two sides of the microvalve). For the 60 nm membrane with constrictions, most pores empty by cavitation at a pressure around 55 mb.

range.

The second method, used at Institut Néel, is a volumetric one. It consists in integrating over time the flowrate $dn/dt$ into the membrane. For a given opening of the microvalve, and at a fixed pressure on the other side of the microvalve (equal to the tank pressure for condensation, and 0 for evaporation), $dn/dt$ is fixed by the (variable) cell pressure $P_{\text{cell}}$. In order to determine $dn/dt(P_{\text{cell}})$, we perform a separate experiment in the exact same conditions without any membrane in the cell. In our experimental conditions, hexane vapor behaves as a perfect gas to better than 1%, so that $dn/dt(P_{\text{cell}}) = RT/V_{\text{cell}}\, dP/dt$, the volume

$V_{\text{cell}}$ (Fig. 3) having been calibrated from a known reference volume. We thus obtain the total mass of hexane in the volume $V_{\text{cell}}$ as a function of pressure. Subtracting the amount of gas outside the membrane yields the liquid mass inside the membrane. In contrast to WLI, the volumetric method probes the full membrane. Thus, the two methods are equivalent only so far condensation or evaporation are homogeneous at the scale of the membrane. Note that the volumetric method does require an integration over time, which makes it more prone to drift errors, hence less precise, especially in the regime of film adsorption. This reason, combined with the time consuming subtraction procedure, explains why we selected WLI for the experiments of Figs.2 and 3 of the paper.

We have compared both methods for the native state of the 60 nm poAl membrane used in the paper (Fig. 2), for which transmission images show that condensation is homogeneous. The sample porosity deduced from the amount of liquid for the filled membrane is 32% for the volumetric method (Fig. 4(b)), close to the 31% above mentioned for WLI. The difference is smaller than the estimated relative error on each measurement. This validates the use of Bruggeman's approximation to quantitatively measure the hexane liquid fraction. The porosity deduced from either measurement has been used to obtain the average pore volume, hence the cavitation rate per unit volume and per unit time (Fig. 4 of the paper).

## DEPENDENCE OF THE EVAPORATION PRESSURE IN POROUS SILICON ON THE CAVITY GEOMETRY

The value of the evaporation pressure of hexane is much larger in poSi than in poAl ink-bottles, confirming the conclusion of Ref.19 for poSi. While this could suggest the occurrence of heterogeneous cavitation, we find that the evaporation pressure depends on the cavity geometry in a much stronger way than would be expected in this case.

Using the construct of Fig 3c of the paper, we have varied the cavity diameter, keeping the constrictions geometry fixed (diameter $\langle d \rangle$=12 nm, length=20 $\mu$m) . We respectively tuned the cavities length $l$ and diameter $\langle d \rangle$ through the thickness and porosity of the bottom layer. We find that $P_{\text{evap}}$ strongly depends on $l$ and $\langle d \rangle$ , ranging from $-12$ MPa for $\langle d \rangle = 26$ nm, $l = 4\,\mu$m, and up to $-6$ MPa for $\langle d \rangle = 50$ nm, $l = 20\,\mu$m. In a standard cavitation scenario, one would expect the cavitation pressure to depend only logarithmically on the cavity volume (for homogeneous cavitation) or surface (for heterogeneous cavitation).

Since the volume (surface) of the cavities changes by a factor 20 (2) at most between the different samples, the strong variation of the evaporation pressure is not consistent with such a standard scenario.

## DETECTION OF CAVITATION IN ALUMINA MEMBRANES BY OPTICAL TRANSMISSION MEASUREMENTS

Condensation and evaporation strongly affect the light transmission through the membrane. This can be monitored at the global membrane scale by illuminating the membrane with a 1 $cm^2$ wide collimated beam of green light and imaging the membrane in transmission with a CCD camera. This is illustrated in Figure 5 for the case of cavitation. Because the membrane strongly scatters at small angles (due to the long pore length), and the CCD objective has a finite aperture, the CCD images also detect a fraction of the scattered light. Pure transmission measurements were thus performed using a He-Ne laser (beam waist $\simeq$ 0.5 mm) and a photodiode 2 meters away.

Fig. 6 compares, for the two membranes of Fig. 4, the volumetric signal to the laser beam transmission relative to the empty state. During the condensation and evaporation phases, corresponding to a quasi-plateau of pressure, a marked dip in transmission is observed for the native membrane. When empty or filled, the membrane scatters light relatively little, resulting in an absolute optical transmission typically above 50%. Although individual pores are strong light scatterers, due to the mismatch of refractive index between alumina and air or hexane, their quite regular organization at a sub-micrometer scale makes the sample homogeneous at the wavelength of light, resulting in this observed good transmission. For the 60 nm membrane, the transmission is larger in the filled state than in the empty state, due to the improved index matching. This is not the case for the 25 nm membrane, which we interpret as a proof that, in this case, some of the pores have been blocked after their formation and cannot fill with liquid. In contrast, when pores are partly filled (as a whole or individually), the homogeneity is lost, leading to large scattering, and a marked drop of transmission [4].

Deposition of constrictions barely affect the condensation volumetric and optical signals, which is expected since the pores still fill from their bottom end. During evaporation, the transmission first decreases down to $P_{\text{cav}} \simeq 55$ mb. This results from the complete

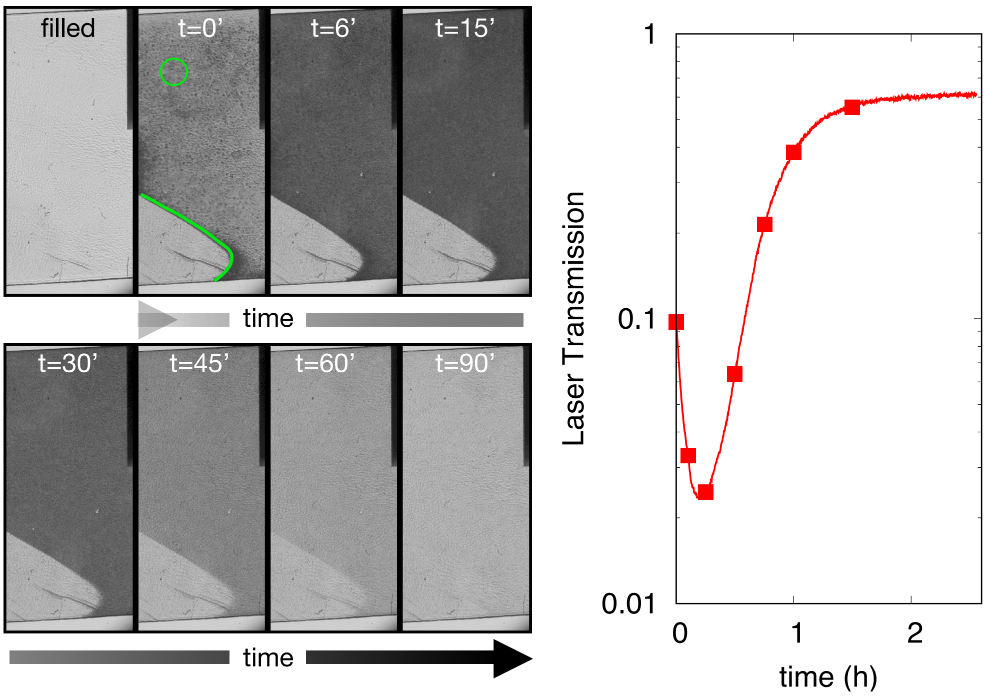


FIG. 5. Transmission images track stochastic cavitation at a constant pressure for the 60 nm poAl membrane. Each image is 1 cm high and has the same logarithmic grey scale. The first image shows the filled (transparent) membrane. The following ones show the temporal evolution following a quench of the reservoir pressure $P_V$ from 60 to 54 mb at time zero. This evolution is homogeneous, except below the green line in the image at time zero. This region, having been protected from the alumina deposition during the formation of constrictions, is already empty at 54 mb. At each point of the remaining of the membrane, a fraction of the pores has an aperture wide enough for having been emptied by meniscus recession above $P_{\text{cav}}$, inducing a loss of transmission at time zero. As cavitation proceeds, the transmission first decreases to a minimum until the fraction of filled pores becomes smaller than 50%, beyond which point it increases again up to the empty membrane value. The graph shows the transmission measured by the laser beam in the circled area on the $t$=0 image, normalized by its value for the filled membrane. Squares correspond to the times of the successive images.

evaporation in the small fraction of pores the aperture of which is large enough to allow meniscus recession. Below this pressure, cavitation sets in, and the number of filled pores decreases. The attenuation first decreases to a minimum, then increases as the fraction of filled pores becomes smaller than 50%, until all pores are empty and the transmission of

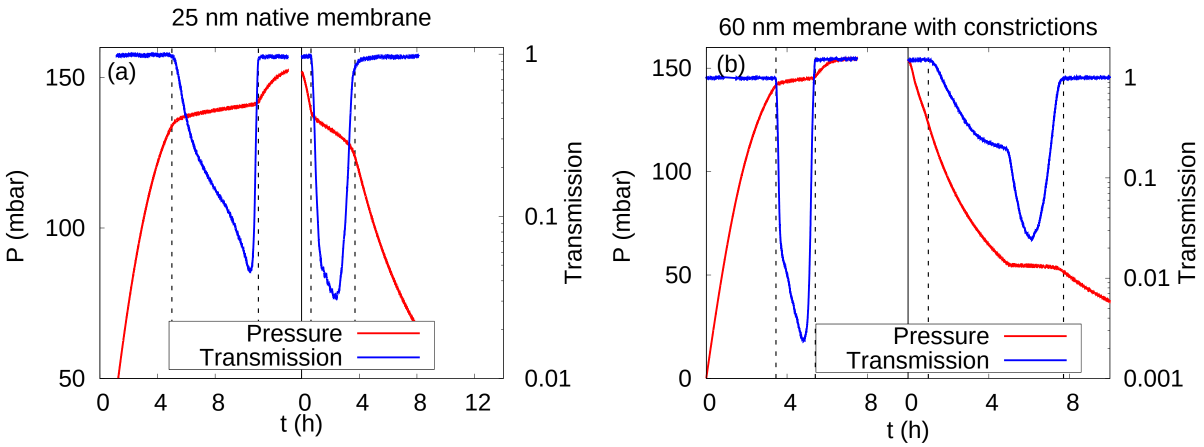


FIG. 6. Time dependence of the cell pressure and transmission during condensation and evaporation, for the same membranes as in Fig. 4. The sample light transmission, measured using a He-Ne laser beam, drops by a large factor during condensation and evaporation in the membrane. Comparison of the volumetric and optical data of Fig. 6(b) shows that, during cavitation, the transmission is minimal when about 50% of the pores are emptied.

the empty membrane is recovered. Transmission images allow to check the uniformity of cavitation throughout the membrane (Figure 5).

In Fig. 7, we thus combine the (global) volumetric and (local) optical informations of Fig. 6b to obtain the relationship between the transmission (relative to the empty state) and the remaining mass of liquid inside the membrane. Analyzis of this figure shows that, in the late stage of cavitation, for transmissions larger than 5%, the logarithm of the transmission relative to the empty state scales with the fraction of still filled pores. Hence, transmission provides an accurate signature of cavitation within the membrane, which can be used as a substitute to volumetric measurements when the latter are not possible.

This is precisely the case when studying the relaxation kinetics of cavitation at a fixed pressure. In these experiments, the microvalve is bypassed and the filled membrane is instantaneously depressurized from $\approx 60$ mbar, at which no cavitation takes place, to the pressure of interest. Due to the stochastic nature of cavitation, different pores empty at different, random, times, and the number of filled pores decreases exponentially with the elapsed time at a rate $\Gamma(P)$. In the late stage of relaxation, the logarithm of the transmission relative to the empty state should scale with this fraction, hence decreases exponentially with time, as we indeed observe. For shorter times, the variation is not exponential (and even non

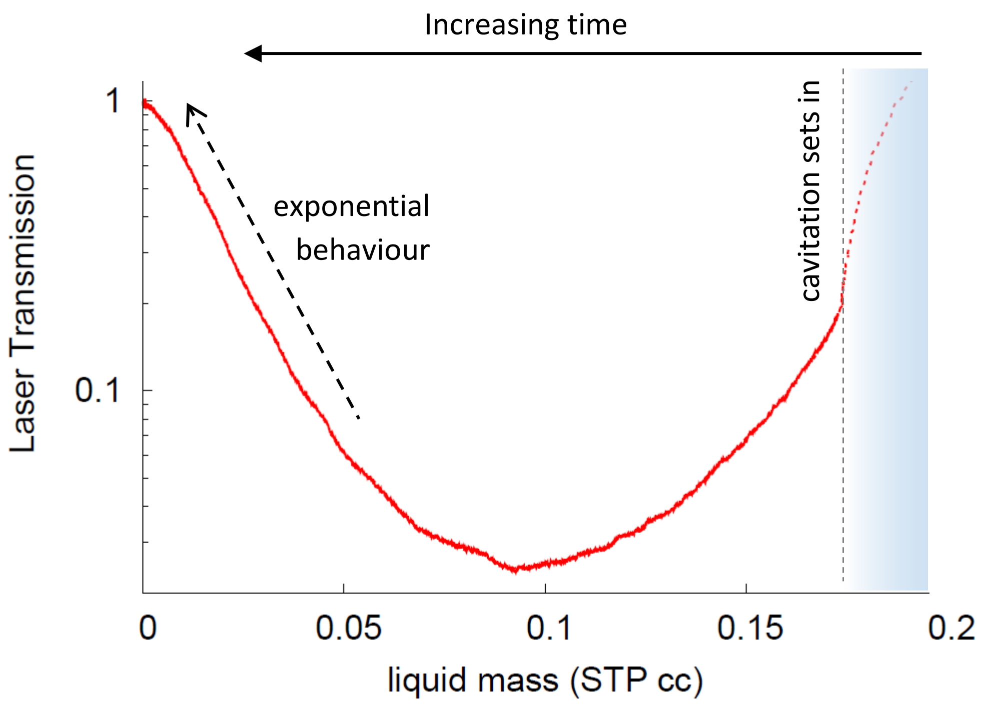


FIG. 7. Relationship between the mass of liquid in the membrane and the laser transmission during evaporation in the experiment of Fig. 6(b). For early times, corresponding to the evaporation in pores with large enough constrictions, the transmission decreases with time, *i.e.* with decreasing mass of liquid (dashed curve). The change of slope around 0.17 STP cm$^3$ reflects the change in the evaporation mechanism, from meniscus recession to cavitation. For smaller masses, pores are either filled or empty, and the transmission keeps on decreasing as the number of empty pores increases. When the mass of liquid is smaller than about half its initial value, more than 50% of the pores are empty and the system is better described as an empty membrane with a fraction of filled pores. As time increases, this fraction decreases and the transmission increases. In the late stage of relaxation, one expects the density of still filled pores to be low enough to enter a single scattering regime, where the logarithm of the transmission varies linearly with their fraction, hence the liquid mass. Such a linear regime is indeed observed for a transmission larger than $\simeq 5\%$.

monotonous), but, from one pressure to the other, the evolution is identical when rescaling the time scale, as illustrated in Fig. 8 for the 25 nm membrane. Fitting the long time behavior with an exponential yields the relaxation rate $\Gamma(P)$ plotted in Fig. 4 of the paper.

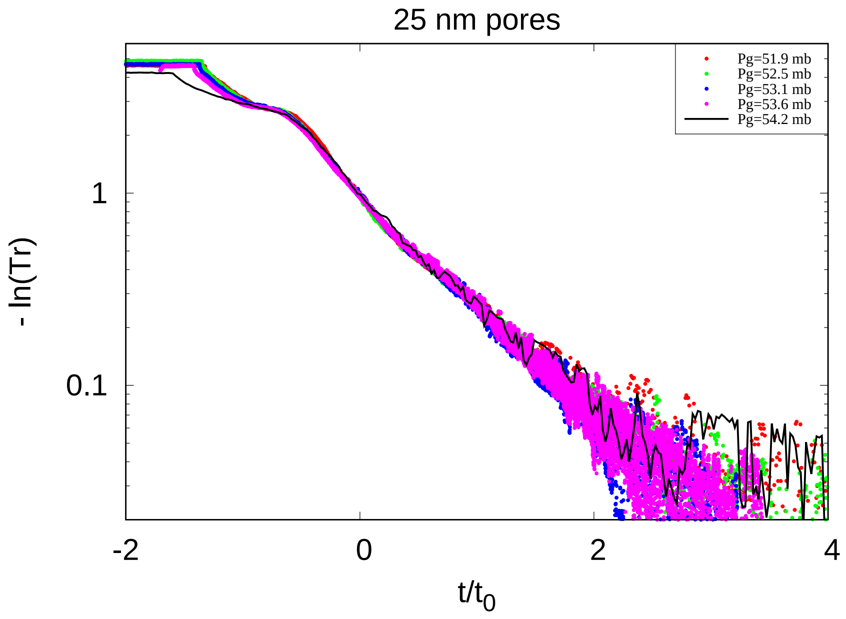


FIG. 8. Kinetics of cavitation in the 25 nm membrane, as followed by the temporal dependence of the transmission of a He-Ne laser beam through the membrane. The time scale is normalized by $t_0$, the measured time interval between transmissions $Tr$=0.38 and 0.77 (relative to the transmission of the empty membrane), time zero corresponding to $Tr$=0.38. Different curves correspond to the pressures indicated in Fig. 4 of the paper. The good collapse demonstrate that the pores empty stochastically, at a rate which only depends on the pressure. The cavitation rate reported in Fig. 4 was obtained by fitting the decay by an exponential in the range ln($Tr$) between $5.10^{-2}$ and 1.

## COMPARISON TO BULK CNT FOR POROUS ALUMINA AND DISCUSSION OF EXPERIMENTAL ERRORS

We have evaluated the effect of confinement on cavitation based on Ref.21 and the van der Waals interaction strength mentionned above (6.4 $10^4$ K.Å$^3$). We find that this effect is negligible for our pore diameters, so that comparison to bulk CNT is meaningful.

In the paper, we conclude that CNT prediction using the bulk surface tension and the usually assumed value for the attempt frequency does not quantitatively account for the

measured pressure dependence of the cavitation rate. Here, we show that this conclusion holds when considering the various experimental errors.

CNT states that the cavitation rate per unit volume $\Gamma$ is given by

$$\Gamma = \Gamma_0 \exp(-E_{\mathrm{b}}/k_{\mathrm{B}}T) \tag{1}$$

with, from Eq.(1) of the paper,

$$E_{\mathrm{b}} = \frac{16\pi\sigma^3}{3\,P_{\mathrm{L}}^2}, \tag{2}$$

since $|P_{\mathrm{L}}| >> P_{\mathrm{V}}$ in our case.

Different expressions have been proposed for the prefactor $\Gamma_0$. Blander and Katz give [22]:

$$\Gamma_0 = n\left(\frac{2\sigma}{\pi M}\right)^{1/2}, \tag{3}$$

with $n$ the density (molecules per unit volume) and $M$ the molecular mass. For hexane, this gives $\Gamma_0 \simeq 2.10^{38}$ m$^{-3}$ s$^{-1}$. Alternatively, Maris [23] has proposed to estimate $\Gamma_0$ as

$$\Gamma_0 = \frac{k_{\mathrm{B}}T}{h}\frac{3}{4\pi R_{\mathrm{c}}^3}, \tag{4}$$

the ratio of a thermal attempt frequency to the volume of the critical germ. $R_{\mathrm{c}}$, the critical radius, of order 2 nm in our experiments, giving $\Gamma_0 \simeq 10^{39}$ m$^{-3}$ s$^{-1}$. These two evaluations agree within an order of magnitude with the value $\Gamma_0$=$2.10^{38}$ m$^{-3}$ s$^{-1}$ taken in the paper, to be compared with the seven orders of magnitude disagreement with CNT when the surface tension is assumed to have its bulk value (0.185 J/m$^2$ at 19°C [24]).

At fixed $\Gamma_0$, and under the latter assumption, the predicted $\Gamma$ in eq.1 is only sensitive to the liquid pressure $P_{\mathrm{L}}$ in eq.2. $P_{\mathrm{L}}$ is derived from the experimentally measured gas pressure $P_{\mathrm{V,cav}}$ at cavitation according to :

$$\mu_{\mathrm{L}}(P_{\mathrm{L}}) = \mu_G(P_{\mathrm{V,cav}}) \tag{5}$$

The values reported in the paper have been computed assuming the liquid to be incompressible - *i.e.* $\mu_{\mathrm{L}}(P_{\mathrm{L}}) = v_L(P_{\mathrm{L}} - P_{\mathrm{sat}})$ with $v_L$ the liquid molar volume taken from NIST data [24] -, and the gas to be perfect - *i.e.* $\mu_G(P_{\mathrm{V,cav}}) = RT\ln(P_{\mathrm{V,cav}}/P_{\mathrm{sat}})$ with $R$ the perfect gas constant- . Using the actual NIST thermodynamic data [24] for the gas increases $|P_{\mathrm{L}}|$ by less than 1%. The effect of the incompressible liquid assumption is more difficult to

assert as $P_L$ lies in the liquid metastable region, for which no data are available. However, assuming either a constant compressibility at negative pressure, or extrapolating the liquid density pressure dependence at positive pressures into the metastable region, both increase $|P_L|$ by less than 2% with respect to the incompressible assumption. Applying these corrections would increase the energy barrier, hence the disagreement between the measured relaxation time and the value expected from standard CNT.

The only way to reconcile our results with the standard CNT would then be an error on $P_{V,cav}/P_{sat}$. In this ratio, $P_{sat}$ is the saturated vapor pressure at the membrane temperature, which could differ from the measured cell temperature, due to thermal exchange between the cell windows and the slightly warmer external air. We checked that the difference cannot exceed 0.2°C, corresponding to a 1% error on $P_{sat}$ ≈155 mb, or a 3% change in the gas chemical potential, hence in the liquid pressure $P_L$. At a constant barrier energy, this corresponds to a change of $\sigma$ of 2%. This is too small compared to the 9% needed to reconcile the measured rates with $\Gamma_0$=2.10$^{38}$ m$^{-3}$ s$^{-1}$.

---

* pierre-etienne.wolf@neel.cnrs.fr, ORCID 0000-0001-8633-7824

† deceased, 2019 August 29th

‡ rolley@phys.ens.fr, ORCID 0000-0003-1333-2541

[1] Masuda H and Fukuda K. Ordered metal nanohole arrays made by a two-step replication of honeycomb structures of anodic alumina. *Science*, **268**, 1466 (1995).

[2] Lee W, Schwirn K, Steinhart M, Pippel E, Scholz R, and Gosele U. Structural engineering of nanoporous anodic aluminium oxide by pulse anodization of aluminium. *Nat. Nano*, **3**, 234 (2008).

[3] Lee W and Park S J. Porous anodic aluminum oxide: Anodization and templated synthesis of functional nanostructures. *Chem. Rev.*, **114**, 7487 (2014).

[4] Doebele V. Condensation et évaporation de l'hexane dans les membranes d'alumine poreuse. Ph.D. thesis, Université Grenoble-Alpes (2019).

[5] Grosman A and Ortega C. Capillary condensation in porous materials. hysteresis and interaction mechanism without pore blocking/percolation process. *Langmuir*, **24**, 3977 (2008).

[6] Grosman A, Puibasset J, and Rolley E. Adsorption-induced strain of a nanoscale silicon

honeycomb. *Europhys. Lett.*, **109**, 56002 (2015).

[7] Rolley E, Garroum N, and Grosman A. Using capillary forces to determine the elastic properties of mesoporous materials. *Phys. Rev. B*, **95**, 064106 (2017).

[8] Bossert M, Grosman A, Trimaille I, Noûs C, and Rolley E. Stress or strain does not impact sorption in stiff mesoporous materials. *Langmuir*, **36**, 11054 (2020).

[9] Zheng Q, Durben D J, Wolf G H, and Angell C A. Liquids at large negative pressures: Water at the homogeneous nucleation limit. *Science*, **254**, 829 (1991).

[10] Azouzi M E M, Ramboz C, Lenain J F, and Caupin F. A coherent picture of water at extreme negative pressure. *Nat. Phys.*, **9**, 38 (2013).

[11] Saam W F and Cole M W. Excitations and thermodynamics for liquid-helium films. *Phys. Rev. B*, **11**, 1086 (1975).

[12] Israelachvili J N. Intermolecular and Surface Forces (Third Edition), (Academic Press, San Diego 2011).

[13] Van Oss C J, Chaudhury M K, and Good R J. Interfacial Lifshitz-Van der Waals and polar interactions in macroscopic systems. *Chem. Rev.*, **88**, 927 (1988).

[14] Puibasset J. Adsorption/desorption hysteresis of simple fluids confined in realistic heterogeneous silica mesopores of micrometric length: A new analysis exploiting a multiscale Monte Carlo approach. *J. Chem. Phys.*, **127**, 154701 (2007).

[15] Bruschi L, Mistura G, Nguyen P T M, Do D D, Nicholson D, Park S J, and Lee W. Adsorption in alumina pores open at one and at both ends. *Nanoscale*, **7**, 2587 (2015).

[16] Morishige K. Nature of adsorption hysteresis in cylindrical pores: Effect of pore corrugation. *J. Phys. Chem. C*, **120**, 22508 (2016).

[17] Pacholski C, Sartor M, Sailor M J, Cunin F, and Miskelly G M. Biosensing using porous silicon double-layer interferometers: Reflective interferometric Fourier transform spectroscopy. *J. Am. Chem. Soc.*, **127**, 11636 (2005).

[18] Casanova F, Chiang C E, Li C P, and Schuller I K. Direct observation of cooperative effects in capillary condensation: The hysteretic origin. *Appl. Phys. Lett.*, **91**, 243103 (2007).

[19] Grosman A and Ortega C. Cavitation in Metastable Fluids Confined to Linear Mesopores. *Langmuir*, **27**, 2364 (2011).

[20] Bruot N and Caupin F. Curvature dependence of the liquid-vapor surface tension beyond the Tolman approximation. *Phys. Rev. Lett.*, **116**, 056102 (2016).

[21] Bonnet F and Wolf P E. Thermally activated condensation and evaporation in cylindrical pores. *J. Phys. Chem. C*, **123**, 1335 (2019).

[22] Blander M and Katz J. Bubble nucleation in liquids. *AIChE Journal*, **21** (1975).

[23] Maris H J and Xiong Q. Nucleation of bubbles in liquid helium at negative pressure. *Phys. Rev. Lett.*, **63**, 1078 (1989).

[24] Lemmon E. W., McLinden M. O. and Friend D. G., "Thermophysical Properties of Fluid Systems" in WebBook of Chemistry NIST, NIST Standard Reference Database SRD Number 69, Eds. P.J. Linstrom and W.G. Mallard, National Institute of Standards and Technology, Gaithersburg MD, 20899, https://doi.org/10.18434/T4D303 , (downloaded April 10th, 2020).
